# Supplementary material for: Rank Overspecified Robust Matrix Recovery: Subgradient Method and Exact Recovery
Source: arXiv:2109.11154 source file (2021-10-26)
Supplement: Supplementary file 1 [file appendixfnorm.tex]

\subsection{Proof of Proposition~\ref{prop: bound on MM NNfnorm}}
By assumption,
\begin{align}
	\norm{S_tS_t^\top} \le \norm{D_S^*} + \norm{S_tS_t^\top - D_S^*} \le 1.01 \sigma_1.
\end{align}
Therefore, $\norm{S_t} \le 2\sqrt{\sigma_1}$. Also,
\begin{align}
	\sigma_r(S_tS_t^\top) \ge \sigma_r(D_S^*) - \norm{S_tS_t^\top -D_S^*} \ge \frac{\sigma_r}{2}.
\end{align}
Hence, $\sigma_r(S_t) \ge \sqrt{\frac{\sigma_r}{2}}$.
\begin{enumerate}
	\item $\fnorm{\cM_t(S_t)\cM_t(S_t)^\top - D^*_S} \le (1-\frac{3\gamma_t\sigma_r}{4}) \fnorm{S_tS_t^\top - D_S^*} + 3 \gamma_t \norm{S_t T_t^\top}^2$.\\
	 By definition,
	\begin{equation}
		\cM_t(S_t)  = S_t - \gamma_t \left(S_t S_t^\top S_t +S_t T_t^\top T_t - D_S^*S_t\right).
	\end{equation}
	This yields
	\begin{align}
		&D_S^* - \cM_t(S_t)\cM_t(S_t)^\top \\
		&=  D_S^* - \left[S_t - \gamma_t \left(S_t S_t^\top S_t +S_t T_t^\top T_t - D_S^*S_t\right)\right]\left[S_t - \gamma_t \left(S_t S_t^\top S_t +S_t T_t^\top T_t - D_S^*S_t\right)\right]^\top\\
		&= Z_1+ Z_2+ Z_3,
	\end{align}
	where 
	\begin{align}
		Z_1 &= D_S^* - S_tS_t^\top  - \gamma_t (D_S^*-S_tS_t^\top )S_tS_t^\top -\gamma_t S_tS_t^\top ( D_S^*-S_tS_t^\top),\\
		Z_2 &= 2\gamma_t S_tT_t^\top T_t S_t^\top ,
	\end{align}
	and 
	\begin{equation}
		Z_3 = -\gamma_t^2 (S_tS_t^\top S_t + S_tT_t^\top T_t - D_S^*S_t)(S_tS_t^\top S_t + S_tT_t^\top T_t - D_S^*S_t)^\top.
	\end{equation}
	We bound each of them separately. For $Z_1$, by triangle inequality,
	\begin{align}
		\fnorm{Z_1} &= \fnorm{\left(D_S^* - S_tS_t^\top\right)\left(\frac{1}{2}I - \gamma_t S_tS_t^\top\right) +\left(\frac{1}{2}I - \gamma_t S_tS_t^\top\right)\left(D_S^* - S_tS_t^\top\right)}\\
		&\le \fnorm{\left(D_S^* - S_tS_t^\top\right)\left(\frac{1}{2}I - \gamma_t S_tS_t^\top\right)} + \fnorm{\left(\frac{1}{2}I - \gamma_t S_tS_t^\top\right)\left(D_S^* - S_tS_t^\top\right)}\\
		&\le \norm{\left(\frac{1}{2}I - \gamma_t S_tS_t^\top\right)}\fnorm{\left(D_S^* - S_tS_t^\top\right)} +\norm{\left(\frac{1}{2}I - \gamma_t S_tS_t^\top\right)}\fnorm{\left(D_S^* - S_tS_t^\top\right)} \\
		&\le  (\frac{1}{2} - \gamma_t \sigma_r^2(S_t))\fnorm{D_S^* -S_tS_t^\top} +(\frac{1}{2} - \gamma_t \sigma_r^2(S_t))\fnorm{D_S^* -S_tS_t^\top}\\
		&\le (1-\gamma_t \sigma_r) \fnorm{D_S^* - S_tS_t^\top}
	\end{align}
	The norm of $Z_2$ can be simply bounded by 
	\begin{equation}
		\norm{Z_2} \le 2\gamma_t \norm{S_t T_t^\top} \fnorm{S_t T_t^\top} \le 2\gamma_t \fnorm{S_t T_t^\top}^2.
	\end{equation}
	For $Z_3$,
	we can split it as 
	\begin{align}
		Z_3 &= - \gamma_t ^2 (S_tS_t^\top - D_S^*)S_tS_t^\top(S_tS_t^\top - D_S^*)^\top  - \gamma_t^2 S_TT_t^\top T_tT_t^\top T_t S_t^\top \\
		&\qquad - \gamma_t^2 \left(S_tT_t^\top T_t\left(S_t^\top S_tS_t^\top -S_t^\top D_S^*\right) + \left(S_tS_t^\top S_t - D_S^*S_t\right)T_t^\top T_t S_t^\top\right)
	\end{align}
	By triangle inequality, 
	\begin{align}
		\norm{Z_3} &\le \gamma_t^2 \norm{S_tS_t^\top-D_S^*}\norm{S_tS_t^\top} \fnorm{S_tS_t^\top -D_S^*} + \gamma_t^2\norm{T_tT_t}^\top \norm{S_tT_t^\top}\fnorm{S_tT_t^\top} \\
		&\qquad+ 2\gamma_t^2\fnorm{S_tS_t^\top -D_S^*} \norm{S_tT_t^\top}^2\\
		&\overset{(\sharp)}{\le} 4\gamma_t^2 \sigma_1 \frac{\sigma_r}{100} \fnorm{S_tS_t^\top - D_S^*} + 0.01 \gamma_t^2\sigma_r \fnorm{S_tT_t^\top}^2 + \gamma_t^2 \sigma_1\sigma_r\fnorm{S_tS_t^\top-D_S^*}\\
			&\le \left(\frac{4}{1000}\gamma_t \sigma_r+\frac{1}{100}\gamma_t \sigma_r\right) \fnorm{S_tS_t^\top - D_S^*} + \gamma_t \fnorm{S_tT_t^\top}^2. 
	\end{align}
	Here $(\sharp)$ follows from our assumption that $\norm{S_tS_t^\top -D_S^*} \le \frac{\sigma_r}{100}$, $\norm{S_t}\le 2\sqrt{\sigma_1}$ and $\norm{T_t} \le 0.1\sqrt{\sigma_r}$.
	Combining, we have
	\begin{align}
		\fnorm{D_S^* - S_{t+1}S_{t+1}^\top} &\le \fnorm{Z_1} + \fnorm{Z_2} + \fnorm{Z_3}\\
		&\le (1-\gamma_t\sigma_r + \frac{21}{100}\gamma_t \sigma_r) \fnorm{D_S^* - S_tS_t^\top} +(2\gamma_t+\gamma_t)\fnorm{S_tT_t^\top}^2\\
		&\le \left(1-\frac{3\gamma_t\sigma_r}{4}\right) \fnorm{D_S^*- S_tS_t^\top} + 3\gamma_t \fnorm{S_tT_t^\top}^2
	\end{align}
	\item $\norm{\cN_t(T_t) \cN_t(T_t)^\top} \le  \norm{T_t}^2(1-\gamma_t \norm{T_t}^2) = \norm{T_tT_t^\top}\left(1-\gamma_t \norm{T_tT_t^\top}\right)$.\\
	By definition, 
	\begin{equation}
		\cN_t(T_t) = T_t - \gamma_t(T_tT_t^\top T_t + T_tS_t^\top S_t).
	\end{equation}
	Plug this into $\cN_t(T_t)\cN_t(T_t)^\top$, we obtain
	\begin{align}
		\cN_t(T_t)\cN_t(T_t)^\top &=  \left(T_t - \gamma_t(T_tT_t^\top T_t + T_tS_t^\top S_t)\right)\left(T_t - \gamma_t(T_tT_t^\top T_t + T_tS_t^\top S_t)\right)^\top\\
		&=Z_4 + Z_5,
	\end{align}
	where 
	\begin{equation}
		Z_4 = T_tT_t^\top -2\gamma_t T_tT_t^\top T_tT_t^\top
	\end{equation}
	and 
	\begin{equation}
		Z_5 =- 2\gamma_t T_tS_t^\top S_tT_t^\top+ \gamma_t^2(T_tT_t^\top T_t + T_tS_t^\top S_t)(T_tT_t^\top T_t + T_tS_t^\top S_t)^\top.
	\end{equation}
	We bound each of them separately. By lemma~\ref{lem: S(I-S) svd}, we obtain
	\begin{align}
		\fnorm{Z_4}&\le \fnorm{T_tT_t^\top - 2\gamma_t T_tT_t^\top T_tT_t^\top}\\
		&\le \norm{I - 2\gamma_t T_tT_t^\top}\fnorm{T_tT_t^\top}\\
		&\le (1-2\gamma_t \norm{T_tT_t^\top})\fnorm{T_tT_t^\top}
	\end{align}
	On the other hand, 
	\begin{align}
		Z_5 &=  - 2\gamma_t T_tS_t^\top S_tT_t^\top + \gamma_t^2\left[T_tT_t^\top \left(T_tS_t^\top S_tT_t^\top \right) + \left(T_tS_t^\top S_tT_t^\top \right) T_tT_t^\top\right] +\gamma_t^2 T_tS_t^\top S_tS_t^\top S_t T_t^\top\\
		&\preceq (-2\gamma_t + \frac{2}{100}\gamma_t^2\sigma_r+ 4\sigma_1\gamma_t^2)T_tS_t^\top S_t T_t^\top\\
		&\preceq 0
	\end{align}
	Combining, we obtain
	\begin{align}
		\fnorm{\cN_t(T_t)\cN_t(T_t)^\top} \le \fnorm{Z_4} \le  (1-2\gamma_t \norm{T_tT_t^\top})\fnorm{T_tT_t^\top}.
	\end{align}
	\item $\norm{\cM_t(S_t)\cN_t(T_t)^\top} \le (1-\frac{\gamma_t\sigma_r}{3})\norm{S_tT_t^\top}$. \\
	By definition of $\cM_t(S_t), \cN_t(T_t)$, we have
	\begin{align}
		\cM_t(S_t) \cN_t(T_t)^\top &= \left(S_t - \gamma_t(S_tS_t^\top S_t + S_t T_t^\top T_t - D_S^* S_t)\right)\left(T_t - \gamma_t(T_tT_t^\top T_t + T_t S_t^\top S_t)\right)^\top\\
		&=Z_6 + Z_7 + Z_8,
	\end{align}
	where 
	\begin{equation}
		Z_6= (I - \gamma_t S_tS_t^\top)S_t T_t^\top,
	\end{equation}
	\begin{equation}
		Z_7 = \gamma_t (D_S^*- S_tS_t^\top)S_tT_t^\top
	\end{equation}
	and 
	\begin{equation}
		Z_8 = -2\gamma_t S_t T_t^\top T_t T_t^\top + \gamma_t^2(S_tS_t^\top S_t + S_t T_t^\top T_t - D_S^* S_t)(T_tT_t^\top T_t + T_tS_t^\top S_t)^\top.
	\end{equation}
	We bound each of them. By our assumption that $\sigma_r(S_t) \ge \sqrt{\frac{\sigma_r}{2}}$, 
	\begin{equation}
		\norm{Z_6} \le (1-\frac{\gamma_t\sigma_r}{2}) \norm{S_tT_t^\top}.
	\end{equation}
	By the assumption that $\norm{D_S^* - S_tS_t^\top} \le \frac{\sigma_r}{10}$, 
	\begin{equation}
		\norm{Z_7}\le \frac{\gamma_t\sigma_r}{10}\norm{S_tT_t^\top}.
	\end{equation}
	For $Z_8$, we use triangle inequality and get 
	\begin{align}
		\norm{Z_8} &\le \norm{2\gamma_t S_t T_t^\top T_t T_t^\top} + \gamma_t^2\norm{(S_tS_t^\top - D_S^*)S_tT_t^\top T_t T_t^\top}\\
		&\qquad +\gamma_t^2\norm{(S_tS_t^\top - D_S^*)S_tS_t^\top S_t T_t^\top)}+ \gamma_t^2 \norm{S_tT_t^\top T_t (T_t^\top T_tT_t^\top + S_t^\top S_t T_t^\top)}\\
		&\overset{(\sharp)}{\le} \frac{2}{100}\gamma_t\sigma_r \norm{S_t T_t^\top} + \gamma_t^2 \frac{\sigma_r}{10}\frac{\sigma_r}{100}\norm{S_tT_T^\top}+4\gamma_t^2 \frac{\sigma_r}{10}\sigma_1\norm{S_tT_t^\top} \\
		&\qquad + \gamma_t^2\left(\frac{\sigma_r}{100}\right)^2 \norm{S_tT_t^\top}+\gamma_t^2\left(\frac{2\sqrt{\sigma_1\sigma_r}}{10}\right)^2 \norm{S_tT_t^\top}\\
		&\overset{(\star)}{\le} \frac{\gamma_t\sigma_r}{20 } \norm{S_t T_t^\top}
	\end{align}
	In $(\sharp)$, we used the bound that $\norm{S_tT_t^\top}\le \norm{S_t}\norm{T_t} \le \frac{2\sqrt{\sigma_1\sigma_r}}{10}$ and $\norm{T_tT_t^\top}\le \frac{\sigma_r}{100}$. $(\star)$ follows from our assumption that $\gamma_t \le \frac{0.01}{\sigma_1}$.
	Combining, we obtain
	\begin{align}
		\norm{\cM_t(S_t)\cN_t(T_t)^\top} &\le \norm{Z_6} + \norm{Z_7} + \norm{Z_8}\\
		&\le \left(1- \frac{\gamma_t\sigma_r}{3}\right) \norm{S_tT_t^\top}.
	\end{align}
\end{enumerate}
